# Supplementary material for: Gaseous argon time projection chamber with electroluminescence enhanced optical readout
Source: arXiv:2212.02385 source file (2023-10-28)
Supplement: Supplementary file 1 [file ZAppendices.tex]

\documentclass[../main.tex]{subfiles}
 
\begin{document}

\section{BlaBlaBla}

\end{document}
